# Supplementary material for: SecBench: A Comprehensive Multi-Dimensional Benchmarking Dataset for LLMs in Cybersecurity
Source: arXiv:2412.20787 source file (2025-01-06)
Supplement: Supplementary file 1 [file appendix_backup.tex]

\subsection{Full Prompt}
\label{appendix:full_prompt}


\noindent \textbf{Code Comprehenstion:}
%

\vspace{+0.6ex}
\noindent\fbox{%
    \parbox{0.46\textwidth}{%
    \footnotesize


I will provide you with a piece of code, which is the implementation of the MPC control algorithm of the Apollo autonomous driving system. Each line of code is offered with the line number and the code content. Please comprehend the provided code and keep them in mind, as I will need you to help me do some analysis of the code.



----------------------

\emph{Code with line numbers.}

----------------------


    }%
    \normalsize
}
\vspace{+0.6ex}



%%%%%%%%%%%%%%%%%%%%%

\noindent \textbf{S1. Control Signal Traceback:}
%

\vspace{+0.6ex}
\noindent\fbox{%
    \parbox{0.46\textwidth}{%
    \footnotesize


\# Task Overview

The provided MPC code performs poorly in simulation, and I need to debug the specific problems. Now look at the following line of code from the provided code:

----------

489:   cmd-$>$set\_acceleration(acceleration\_cmd);

----------

This line of code will set the acceleration to the value of variable `acceleration\_cmd'. Now I need you to do a backward data flow analysis, starting from the above line of code (489:   cmd-$>$set\_acceleration(acceleration\_cmd);), to track how this `acceleration\_cmd' is derived.


\# Detailed Requirement

Specifically, you should conduct the following analysis:

1. Conduct the backward data flow analysis to determine which lines of code are related to the calculation of `acceleration\_cmd'.

2. Comprehend the functionality of the identified code and explain why these lines of code are involved in the calculation.


\# Output Format

Accordingly, your output should follow the following format:

*****

Involved code - Line number: Code content

Explanation - The functionality of the involved code (i.e., how this code contributes to the calculation).

*****

Involved code - ...

Explanation - ...

...


    }%
    \normalsize
}
\vspace{+0.6ex}



%%%%%%%%%%%%%%%%%%%%%%%%%%%%%

\noindent \textbf{S2. Interactive Querying - Bug Location Pinpointing:}
%


\vspace{+0.6ex}
\noindent\fbox{%
    \parbox{0.46\textwidth}{%
    \footnotesize


The provided MPC controller code is tested with the Carla simulator. Unfortunately, I found that the controller performs poorly and cannot follow the planned trajectory. It is possible that the provided contains several bugs that lead to such under-performance.

Based on your observation, and the result of your previous code analysis, please carefully examine the provided code, and identify the bugs within.


Your output should follow the following format:


*****

Possibly buggy code - Line number: Code content

Explanation - Why this code is buggy and will lead to under-performance of the controller.

*****

Involved code - ...

Explanation - ...

...



    }%
    \normalsize
}
\vspace{+0.6ex}


\noindent \textbf{S2. Interactive Querying - Potential Issue Highlighting:}
%

\vspace{+0.6ex}
\noindent\fbox{%
    \parbox{0.46\textwidth}{%
    \footnotesize

Now I need you to give me some suggestions on debugging these codes. Based on your observation, and the result of your previous code analysis, please carefully examine the provided code, and tell me ``which part of the code'' could be buggy which I need to pay extra attention to.


    }%
    \normalsize
}
\vspace{+0.6ex}



\noindent \textbf{S2. Interactive Querying - Cross-Module Insights:}
%

\vspace{+0.6ex}
\noindent\fbox{%
    \parbox{0.46\textwidth}{%
    \footnotesize

The autonomous driving system is complex and consists of many different modules (e.g., localization, perception, planning, control...). As a result, it is possible that such under-performance is due to the insufficiency of other modules. Based on your observation, and the result of your previous code analysis, please carefully examine the provided code, and give me suggestions on what other modules that could affect the control performance, which I need to pay extra attention to.

    }%
    \normalsize
}
\vspace{+0.6ex}


%%%%%%%%%%%%%%%%%%%%%%%%%%%%%%




\subsection{Oracle-based Assessment: Detailed Data}
\label{appendix:detailed_TE}

This section shows the full data of the oracle-based assessment in \S\ref{subsec:basic_assessment}.
%
Specifically, Tab.\ref{tab:detailed_tracking_error}, Tab.\ref{tab:O2_detail}, Tab.\ref{tab:O3_detail} and Tab.\ref{tab:O4_detail} corresponds to Tab.\ref{tab:TE_Error}, Tab.\ref{tab:O2}, Tab.\ref{tab:O3} and Tab.\ref{tab:O4}, respectively.


\begin{table*}[h]
    \centering
    \caption{\textbf{O1: Tracking Error between the planned trajectory and actual trajectory.} $e_{p,max}$: maximum position error; $\bar{e}_p$: average position error; $e_{\theta,max}$: maximum $\theta$ error; $\bar{e}_{\theta}$: average $\theta$ error; $e_{v,max}$ : maximum velocity error; $\bar{e}_v$: average velocity error; $e_{a,max}$ : maximum acceleration error; $\bar{e}_a$: average acceleration error. The percentage after $e_{v,max}$, $\bar{e}_v$, $e_{a,max}$, $\bar{e}_a$ show the percentage of how much this error is based on the average state value.}
    \vspace{-2ex}
    \label{tab:detailed_tracking_error}
    \scalebox{0.72}{
    \begin{tabular}{lccccccccccc}
        \toprule
        & \multicolumn{3}{c}{Means} & \multicolumn{2}{c}{Position Error ($m$)} & \multicolumn{2}{c}{$\theta$ Error ($degree$)} & \multicolumn{2}{c}{$v$ Error ($m/s$)} & \multicolumn{2}{c}{$a$ Error ($m^{2}/s$) } \\
        \cmidrule(r){2-4} \cmidrule(lr){5-6} \cmidrule(lr){7-8} \cmidrule(lr){9-10} \cmidrule(l){11-12}
        & $\bar{\theta}$ & $\bar{v}$ & $\bar{a}$ & $e_{p,max}$ & $\bar{e}_p$ & $e_{\theta,max}$ & $\bar{e}_{\theta}$ & $e_{v,max}$ & $\bar{e}_v$ & $e_{a,max}$ & $\bar{e}_a$ \\
        \midrule
        B1\_01 & 89.84 & 1.44 & -0.00078 & 3.83 & 1.24 & 0.88 & 0.07 & (2.25, 156.37\%) & (0.81, 56.31\%) & (2.19, 280212.60\%) & (0.89, 113315.58\%) \\
        B1\_02 & 87.84 & 0.92 & 0.0017 & 3.50 & 1.18 & 6.35 & 0.44 & (1.93, 209.62\%) & (0.82, 88.56\%) & (2.13, 124860.78\%) & (0.65, 37952.42\%) \\
        B1\_03 & 90.80 & 1.01 & 0.00312 & 3.56 & 1.23 & 1.56 & 0.16 & (1.80, 178.18\%) & (0.90, 88.83\%) & (1.89, 60555.80\%) & (0.72, 23018.73\%) \\
        B1\_04 & 90.44 & 1.92 & 0.00745 & 3.40 & 1.00 & 0.48 & 0.07 & (2.29, 119.14\%) & (0.85, 44.07\%) & (4.02, 53957.33\%) & (1.05, 14131.32\%) \\
        B1\_05 & 90.31 & 1.74 & 0.00611 & 3.08 & 1.05 & 0.17 & 0.04 & (1.76, 101.00\%) & (0.83, 47.46\%) & (6.91, 113090.04\%) & (1.07, 17549.31\%) \\
        B1\_06 & 90.36 & 1.98 & -0.00002 & 3.37 & 1.11 & 0.26 & 0.04 & (2.05, 103.50\%) & (0.82, 41.32\%) & (2.11, 13069891.87\%) & (1.13, 7011850.13\%) \\
        \textbf{B1\_mean} & \textbackslash & \textbackslash & \textbackslash & \textbf{3.46} & \textbf{1.14} & \textbf{1.62} & \textbf{0.14} & \textbf{(2.01, 144.64\%)} & \textbf{(0.84, 61.09\%)} & \textbf{(3.21, 2283761.40\%)} & \textbf{(0.92, 1202970.00\%)} \\
        \hline
        B2\_01 & 131.08 & 0.64 & 0.02284 & 3.20 & 0.62 & 17.04 & 2.04 & (1.92, 299.46\%) & (0.73, 114.06\%) & (5.94, 26022.73\%) & (0.55, 2398.25\%) \\
        B2\_02 & 91.93 & 1.44 & 0.03343 & 3.10 & 1.08 & 9.82 & 0.73 & (2.73, 189.54\%) & (0.93, 64.57\%) & (1.96, 5868.67\%) & (0.90, 2695.51\%) \\
        B2\_03 & 120.23 & 1.19 & 0.07833 & 3.35 & 1.11 & 15.65 & 1.78 & (2.74, 229.99\%) & (0.84, 70.04\%) & (5.31, 6773.36\%) & (0.82, 1046.92\%) \\
        B2\_04 & 91.24 & 1.42 & 0.01986 & 2.86 & 1.00 & 3.10 & 0.27 & (2.23, 156.58\%) & (0.90, 63.32\%) & (1.92, 9642.56\%) & (0.90, 4532.59\%) \\
        B2\_05 & 91.53 & 1.44 & 0.03629 & 3.21 & 1.02 & 7.65 & 0.56 & (1.93, 134.05\%) & (0.89, 62.03\%) & (1.81, 4985.60\%) & (0.87, 2390.34\%) \\
        B2\_06 & 91.61 & 1.73 & 0.02708 & 3.12 & 1.03 & 10.11 & 0.39 & (3.08, 178.13\%) & (0.86, 49.97\%) & (2.14, 7892.12\%) & (0.93, 3417.89\%) \\
        \textbf{B2\_mean} & \textbackslash & \textbackslash & \textbackslash & \textbf{3.14} & \textbf{0.98} & \textbf{10.56} & \textbf{0.96} & \textbf{(2.44, 197.96\%)} & \textbf{(0.86, 70.67\%)} & \textbf{(3.18, 10197.51\%)} & \textbf{(0.83, 2746.92\%)} \\
        \hline
        B3\_01 & 89.67 & 1.41 & -0.01227 & 3.20 & 1.18 & 12.41 & 0.52 & (3.40, 241.71\%) & (0.99, 70.15\%) & (2.50, 20407.59\%) & (1.01, 8230.50\%) \\
        B3\_02 & 48.80 & 0.50 & -0.19395 & 3.44 & 1.04 & 29.31 & 4.65 & (2.60, 520.82\%) & (0.67, 134.03\%) & (17.62, 9082.46\%) & (0.84, 435.01\%) \\
        B3\_03 & 79.42 & 0.87 & -0.04143 & 3.34 & 1.10 & 28.98 & 2.96 & (1.90, 219.50\%) & (0.95, 109.47\%) & (15.42, 37228.48\%) & (1.10, 2648.54\%) \\
        B3\_04 & 68.66 & 0.81 & -0.19882 & 3.34 & 0.90 & 25.95 & 3.35 & (2.96, 365.46\%) & (0.75, 92.68\%) & (13.08, 6579.88\%) & (1.04, 521.17\%) \\
        B3\_05 & 89.72 & 1.16 & -0.00049 & 2.91 & 1.02 & 3.27 & 0.35 & (1.76, 152.46\%) & (0.91, 78.84\%) & (2.10, 427807.39\%) & (0.94, 192681.98\%) \\
        B3\_06 & 90.48 & 1.30 & 0.00788 & 3.02 & 1.08 & 5.69 & 0.30 & (2.96, 228.40\%) & (0.89, 68.82\%) & (2.41, 30584.20\%) & (0.93, 11796.99\%) \\
        \textbf{B3\_mean} & \textbackslash & \textbackslash & \textbackslash & \textbf{3.21} & \textbf{1.05} & \textbf{17.60} & \textbf{2.02} & \textbf{(2.60, 288.06\%)} & \textbf{(0.86, 92.33\%)} & \textbf{(8.85, 88615.00\%)} & \textbf{(0.98, 36052.36\%)} \\
        \hline
        B4\_01 & 123.34 & 1.63 & 0.05428 & 3.01 & 1.08 & 2.54 & 0.55 & (3.09, 190.00\%) & (0.83, 50.80\%) & (3.35, 6175.23\%) & (1.10, 2035.51\%) \\
        B4\_02 & 117.33 & 1.93 & 0.07130 & 2.87 & 1.06 & 2.50 & 0.36 & (1.95, 101.44\%) & (0.78, 40.61\%) & (4.45, 6238.54\%) & (1.08, 1515.02\%) \\
        B4\_03 & 140.65 & 1.93 & 0.05235 & 2.89 & 1.06 & 2.28 & 0.27 & (2.85, 147.66\%) & (0.77, 39.90\%) & (2.65, 5061.21\%) & (1.09, 2075.94\%) \\
        B4\_04 & 134.37 & 1.77 & 0.05393 & 3.26 & 1.22 & 2.93 & 0.39 & (3.17, 179.18\%) & (0.68, 38.22\%) & (2.58, 4779.05\%) & (1.13, 2098.15\%) \\
        B4\_05 & 115.95 & 1.36 & 0.04932 & 2.96 & 1.19 & 4.50 & 0.67 & (2.56, 188.24\%) & (0.86, 63.42\%) & (2.92, 5926.72\%) & (1.18, 2397.73\%) \\
        B4\_06 & 119.78 & 1.20 & 0.02909 & 2.98 & 1.20 & 5.81 & 0.66 & (3.09, 256.30\%) & (0.88, 72.96\%) & (3.11, 10699.64\%) & (1.11, 3814.93\%) \\
        \textbf{B4\_mean} & \textbackslash & \textbackslash & \textbackslash & \textbf{2.99} & \textbf{1.14} & \textbf{3.43} & \textbf{0.48} & \textbf{(2.79, 177.14\%)} & \textbf{(0.80, 50.98\%)} & \textbf{(3.18, 6480.07\%)} & \textbf{(1.12, 2322.88\%)} \\
        \hline
        B5\_01 & 77.55 & 1.81 & -0.07108 & 2.73 & 1.02 & 2.77 & 0.55 & (3.18, 175.50\%) & (0.79, 43.35\%) & (2.18, 3073.71\%) & (1.10, 1541.50\%) \\
        B5\_02 & 78.48 & 1.69 & -0.05581 & 2.77 & 1.00 & 2.49 & 0.51 & (3.10, 183.77\%) & (0.84, 49.73\%) & (3.16, 5654.29\%) & (1.12, 2014.45\%) \\
        B5\_03 & 77.29 & 1.86 & -0.07268 & 2.69 & 1.00 & 2.27 & 0.40 & (1.88, 100.88\%) & (0.80, 42.84\%) & (2.39, 3287.65\%) & (1.10, 1512.53\%) \\
        B5\_04 & 61.71 & 1.38 & -0.05407 & 2.93 & 1.21 & 2.95 & 0.62 & (3.07, 221.74\%) & (0.83, 60.10\%) & (2.78, 5134.57\%) & (1.14, 2101.38\%) \\
        B5\_05 & 59.82 & 1.26 & -0.03823 & 2.98 & 1.11 & 2.75 & 0.45 & (2.37, 188.35\%) & (0.77, 60.94\%) & (3.34, 8736.97\%) & (1.06, 2772.06\%) \\
        B5\_06 & 61.12 & 1.34 & -0.04352 & 2.94 & 1.16 & 2.65 & 0.59 & (3.05, 226.74\%) & (0.80, 59.64\%) & (3.38, 7772.93\%) & (1.10, 2519.73\%) \\
        \textbf{B5\_mean} & \textbackslash & \textbackslash & \textbackslash & \textbf{2.84} & \textbf{1.08} & \textbf{2.65} & \textbf{0.52} & \textbf{(2.78, 182.83\%)} & \textbf{(0.80, 52.77\%)} & \textbf{(2.87, 5610.02\%)} & \textbf{(1.10, 2076.94\%)} \\
        \hline
        \textbf{Overall\_mean} & \textbackslash & \textbackslash & \textbackslash & \textbf{3.13} & \textbf{1.08} & \textbf{7.17} & \textbf{0.82} & \textbf{(2.52, 198.13\%)} & \textbf{(0.83, 65.57\%)} & \textbf{(4.26, 478932.80\%)} & \textbf{(0.99, 249233.82\%)} \\
        \bottomrule
    \end{tabular}
    }
\end{table*}



\begin{table*}[h]
\centering
\centering
\caption{\textbf{O2:} Responsiveness assessment of all basic scenarios.}
\label{tab:O2_detail}
\vspace{-2ex}
\scalebox{0.92}{
\begin{tabular}{lcccccccccccc}
\toprule
& \multicolumn{3}{c}{Position} & \multicolumn{3}{c}{\( \theta \)} & \multicolumn{3}{c}{\( v \)} & \multicolumn{3}{c}{\( a \)} \\
\cmidrule(lr){2-4} \cmidrule(lr){5-7} \cmidrule(lr){8-10} \cmidrule(lr){11-13}
& \( FR \) & \( \bar{t}_s \) & \( t_{s,max} \) & \( FR \) & \( \bar{t}_s \) & \( t_{s,max} \) &  \( FR \) & \( \bar{t}_s \) & \( t_{s,max} \) &  \( FR \) & \( \bar{t}_s \) & \( t_{s,max} \) \\
\midrule
B1\_01 & 4.42\% & 2.14s & 17.39s & \textbackslash & \textbackslash & \textbackslash & 75.41\% & 4.53s & 107.68s & 62.95\% & 20.83s & 164.17s \\
B1\_02 & 10.40\% & 2.45s & 12.84s & \textbackslash & \textbackslash & \textbackslash & 77.27\% & 6.30s & 53.03s & 46.76\% & 14.30s & 72.79s \\
B1\_03 & 7.26\% & 2.43s & 11.52s & \textbackslash & \textbackslash & \textbackslash & 84.85\% & 1.24s & 6.94s & 64.79\% & 12.67s & 56.50s \\
B1\_04 & 1.73\% & 0.76s & 3.51s & \textbackslash & \textbackslash & \textbackslash & 56.21\% & 1.93s & 26.62s & 37.45\% & 18.13s & 58.39s \\
B1\_05 & 5.61\% & 0.80s & 2.75s & \textbackslash & \textbackslash & \textbackslash & 66.46\% & 1.19s & 6.56s & 83.23\% & 0.48s & 7.28s \\
B1\_06 & 2.01\% & 0.85s & 3.80s & \textbackslash & \textbackslash & \textbackslash & 63.06\% & 2.14s & 69.07s & 85.43\% & 8.25s & 63.91s \\
\textbf{B1\_mean} & \textbf{5.24\%} & \textbf{1.57s} & \textbf{8.63s} & \textbackslash & \textbackslash & \textbackslash & \textbf{70.54\%} & \textbf{2.89s} & \textbf{44.98s} & \textbf{63.44\%} & \textbf{12.44s} & \textbf{70.51s} \\
\hline
B2\_01 & 27.08\% & 0.40s & 3.47s & 28.90\% & 0.57s & 39.03s & 85.17\% & 6.13s & 14.83s & 2.72\% & 6.97s & 57.89s \\
B2\_02 & 5.94\% & 0.93s & 4.23s & 9.30\% & 0.79s & 4.59s & 65.38\% & 1.49s & 8.13s & 72.79\% & 5.22s & 18.65s \\
B2\_03 & 27.46\% & 0.82s & 4.51s & 0.00\% & 0.39s & 4.67s & 69.56\% & 1.24s & 39.13s & 23.85\% & 8.35s & 32.19s \\
B2\_04 & 4.95\% & 0.88s & 3.49s & 16.37\% & 0.95s & 5.38s & 63.95\% & 1.67s & 15.33s & 74.78\% & 2.61s & 13.14s \\
B2\_05 & 6.96\% & 0.85s & 3.43s & 6.42\% & 0.29s & 2.66s & 68.47\% & 1.10s & 10.00s & 82.77\% & 3.21s & 17.52s \\
B2\_06 & 4.47\% & 0.78s & 3.75s & 3.77\% & 0.18s & 2.15s & 66.78\% & 1.26s & 37.16s & 56.10\% & 10.15s & 35.78s \\
\textbf{B2\_mean} & \textbf{12.81\%} & \textbf{0.78s} & \textbf{3.81s} & \textbf{10.79\%} & \textbf{0.53s} & \textbf{9.75s} & \textbf{69.88\%} & \textbf{2.15s} & \textbf{20.76s} & \textbf{52.17\%} & \textbf{6.08s} & \textbf{29.19s} \\
\hline
B3\_01 & 6.32\% & 1.26s & 5.81s & 1.72\% & 0.34s & 5.19s & 70.45\% & 2.81s & 47.02s & 58.50\% & 21.84s & 60.93s \\
B3\_02 & 58.55\% & 1.17s & 8.09s & 46.19\% & 1.29s & 41.17s & 77.21\% & 3.12s & 27.59s & 0.06\% & 3.28s & 51.63s \\
B3\_03 & 21.26\% & 1.23s & 5.51s & 5.00\% & 0.67s & 5.38s & 65.60\% & 1.98s & 20.60s & 21.19\% & 7.03s & 33.90s \\
B3\_04 & 33.06\% & 1.04s & 6.24s & 27.95\% & 1.01s & 12.55s & 69.68\% & 2.49s & 24.87s & 3.90\% & 6.64s & 35.71s \\
B3\_05 & 7.21\% & 1.21s & 6.92s & 12.72\% & 1.52s & 8.57s & 65.21\% & 2.07s & 15.94s & 65.28\% & 8.78s & 26.78s \\
B3\_06 & 4.58\% & 1.15s & 4.88s & 10.11\% & 1.22s & 12.59s & 70.17\% & 1.65s & 28.40s & 75.09\% & 2.88s & 15.07s \\
\textbf{B3\_mean} & \textbf{21.83\%} & \textbf{1.18s} & \textbf{6.24s} & \textbf{17.28\%} & \textbf{1.01s} & \textbf{14.24s} & \textbf{69.72\%} & \textbf{2.35s} & \textbf{27.40s} & \textbf{37.34\%} & \textbf{8.41s} & \textbf{37.34s} \\
\hline
B4\_01 & 6.32\% & 1.05s & 8.14s & 2.50\% & 0.39s & 10.58s & 64.51\% & 2.48s & 72.87s & 15.90\% & 10.49s & 57.70s \\
B4\_02 & 4.71\% & 0.83s & 4.82s & 0.55\% & 0.14s & 1.74s & 42.94\% & 11.04s & 65.19s & 38.82\% & 7.48s & 43.29s \\
B4\_03 & 1.88\% & 0.84s & 4.28s & 0.41\% & 0.12s & 5.64s & 61.36\% & 2.46s & 108.29s & 51.67\% & 6.84s & 51.19s \\
B4\_04 & 2.28\% & 1.49s & 8.06s & 0.07\% & 0.17s & 3.66s & 60.83\% & 2.71s & 149.91s & 57.32\% & 9.68s & 70.59s \\
B4\_05 & 6.53\% & 1.92s & 8.26s & 0.03\% & 0.62s & 13.49s & 51.70\% & 7.94s & 55.99s & 36.88\% & 13.96s & 136.84s \\
B4\_06 & 12.46\% & 2.05s & 12.00s & 8.00\% & 0.55s & 19.45s & 58.74\% & 6.44s & 65.48s & 28.99\% & 17.33s & 146.15s \\
\textbf{B4\_mean} & \textbf{5.70\%} & \textbf{1.36s} & \textbf{7.59s} & \textbf{1.93\%} & \textbf{0.33s} & \textbf{9.09s} & \textbf{56.68\%} & \textbf{5.51s} & \textbf{86.29s} & \textbf{38.26\%} & \textbf{10.96s} & \textbf{84.29s} \\
\hline
B5\_01 & 3.04\% & 0.75s & 4.82s & 0.78\% & 0.28s & 1.67s & 56.90\% & 1.42s & 36.13s & 60.75\% & 5.58s & 32.94s \\
B5\_02 & 6.45\% & 0.72s & 3.61s & 5.28\% & 0.30s & 2.39s & 56.68\% & 2.43s & 24.99s & 55.14\% & 7.07s & 30.91s \\
B5\_03 & 3.63\% & 0.73s & 2.56s & 1.27\% & 0.24s & 1.62s & 64.01\% & 1.65s & 28.61s & 66.28\% & 3.98s & 21.07s \\
B5\_04 & 13.45\% & 1.73s & 9.40s & 1.60\% & 0.38s & 8.81s & 71.82\% & 1.85s & 64.88s & 25.88\% & 23.95s & 87.39s \\
B5\_05 & 11.44\% & 1.60s & 8.43s & 1.58\% & 0.26s & 2.66s & 61.31\% & 2.22s & 59.79s & 22.83\% & 22.43s & 100.08s \\
B5\_06 & 10.13\% & 1.86s & 11.31s & 0.24\% & 0.65s & 12.12s & 53.29\% & 9.14s & 66.01s & 19.16\% & 24.01s & 99.41s \\
\textbf{B5\_mean} & \textbf{8.02\%} & \textbf{1.23s} & \textbf{6.69s} & \textbf{1.79\%} & \textbf{0.35s} & \textbf{4.88s} & \textbf{60.67\%} & \textbf{3.12s} & \textbf{46.74s} & \textbf{41.67\%} & \textbf{14.50s} & \textbf{61.97s} \\
\hline
\textbf{Overall\_mean} & \textbf{10.72\%} & \textbf{1.22s} & \textbf{6.59s} & \textbf{7.95\%} & \textbf{0.56s} & \textbf{9.49s} & \textbf{65.50\%} & \textbf{3.20s} & \textbf{45.23s} & \textbf{46.58\%} & \textbf{10.48s} & \textbf{56.66s} \\
\bottomrule
\end{tabular}
}
\end{table*}








\begin{table}[ht]
\centering
\caption{\textbf{O3: Stability assessment based on the derivatives of the defined Lyapunov function.} $\bar{\dot{V}}$: Average derivative of the Lyapunov function value; $\dot{V}_{max}$: Maximum derivative. }
\label{tab:O3_detail}
\vspace{-2ex}
\scalebox{0.66}{
\begin{tabular}{lcccccccc}
\toprule
& \multicolumn{2}{c}{Position ($m/s$)} & \multicolumn{2}{c}{\( \theta \) ($degree/s$)} & \multicolumn{2}{c}{\( v \) ($m/s^{2}$)} & \multicolumn{2}{c}{\( a \) ($m/s^{3}$)} \\
\cmidrule(lr){2-3} \cmidrule(lr){4-5} \cmidrule(lr){6-7} \cmidrule(lr){8-9}
& \( \bar{\dot{V}} \) & \( \dot{V}_{max} \) & \( \bar{\dot{V}} \) & \( \dot{V}_{max} \) & \( \bar{\dot{V}} \) & \( \dot{V}_{max} \) & \( \bar{\dot{V}} \) & \( \dot{V}_{max} \)  \\
\midrule
B1\_01 & -0.043 & 3.646 & \textbackslash & \textbackslash & -0.024 & 2.328 & -0.011 & 13.806 \\ 
B1\_02 & 0.099 & 3.225 & \textbackslash & \textbackslash & 0.047 & 2.283 & -0.020 & 12.119 \\ 
B1\_03 & -0.010 & 3.148 & \textbackslash & \textbackslash & -0.002 & 2.120 & -0.006 & 7.166 \\ 
B1\_04 & -0.095 & 3.582 & \textbackslash & \textbackslash & -0.057 & 3.708 & -0.042 & 31.347 \\ 
B1\_05 & -0.132 & 3.118 & \textbackslash & \textbackslash & -0.085 & 2.206 & -0.167 & 48.391 \\ 
B1\_06 & -0.061 & 3.515 & \textbackslash & \textbackslash & -0.033 & 2.249 & -0.010 & 15.101 \\ 
\textbf{B1\_mean} & \textbf{-0.040} & \textbf{3.372} & \textbackslash & \textbackslash & \textbf{-0.026} & \textbf{2.482} & \textbf{-0.043} & \textbf{21.322} \\ 
B2\_01 & -0.075 & 2.937 & 0.095 & 37.912 & -0.032 & 1.974 & -0.038 & 76.632 \\ 
B2\_02 & 0.004 & 3.100 & 0.123 & 16.704 & 0.056 & 2.010 & 0.046 & 20.707 \\ 
B2\_03 & -0.172 & 2.951 & -0.407 & 25.968 & -0.147 & 1.908 & -0.078 & 46.556 \\ 
B2\_04 & -0.012 & 2.923 & 0.059 & 4.883 & 0.016 & 1.671 & 0.013 & 12.791 \\ 
B2\_05 & -0.114 & 2.961 & -0.064 & 13.377 & 0.013 & 1.843 & 0.025 & 20.576 \\ 
B2\_06 & -0.173 & 3.408 & -0.022 & 17.609 & -0.103 & 2.305 & -0.050 & 17.440 \\ 
\textbf{B2\_mean} & \textbf{-0.090} & \textbf{3.047} & \textbf{-0.036} & \textbf{19.409} & \textbf{-0.033} & \textbf{1.952} & \textbf{-0.014} & \textbf{32.450} \\ 
B3\_01 & -0.006 & 3.582 & 0.203 & 35.525 & 0.032 & 2.384 & -0.037 & 25.200 \\ 
B3\_02 & 0.006 & 4.256 & 0.118 & 86.572 & 0.060 & 5.009 & -0.067 & 148.707 \\ 
B3\_03 & -0.064 & 2.619 & -0.364 & 41.169 & 0.094 & 2.013 & -0.221 & 145.122 \\ 
B3\_04 & 0.003 & 3.093 & 0.164 & 33.071 & 0.059 & 8.397 & 0.046 & 133.937 \\ 
B3\_05 & 0.086 & 2.914 & 0.038 & 3.141 & 0.088 & 2.122 & 0.011 & 17.353 \\ 
B3\_06 & -0.207 & 2.961 & -0.025 & 9.117 & -0.156 & 2.200 & 0.032 & 38.535 \\ 
\textbf{B3\_mean} & \textbf{-0.030} & \textbf{3.238} & \textbf{0.022} & \textbf{34.766} & \textbf{0.029} & \textbf{3.687} & \textbf{-0.039} & \textbf{84.809} \\ 
B4\_01 & -0.076 & 3.310 & -0.039 & 4.328 & -0.051 & 2.623 & -0.028 & 37.081 \\ 
B4\_02 & -0.068 & 5.890 & -0.039 & 6.304 & -0.105 & 3.624 & 0.023 & 29.101 \\ 
B4\_03 & -0.102 & 3.538 & -0.034 & 3.827 & -0.142 & 2.331 & -0.064 & 17.638 \\ 
B4\_04 & -0.055 & 3.312 & -0.018 & 3.746 & -0.101 & 2.216 & -0.024 & 8.093 \\ 
B4\_05 & -0.021 & 3.436 & -0.024 & 4.629 & -0.044 & 2.230 & -0.002 & 15.252 \\ 
B4\_06 & -0.026 & 3.424 & -0.001 & 6.220 & -0.049 & 2.284 & 0.006 & 19.753 \\ 
\textbf{B4\_mean} & \textbf{-0.058} & \textbf{3.818} & \textbf{-0.026} & \textbf{4.843} & \textbf{-0.082} & \textbf{2.551} & \textbf{-0.015} & \textbf{21.153} \\ 
B5\_01 & -0.057 & 3.693 & -0.005 & 3.540 & -0.117 & 2.364 & 0.053 & 21.775 \\ 
B5\_02 & -0.088 & 3.365 & -0.063 & 3.623 & -0.080 & 2.269 & 0.002 & 34.080 \\ 
B5\_03 & -0.087 & 3.260 & -0.077 & 3.177 & -0.036 & 2.076 & -0.017 & 23.872 \\ 
B5\_04 & 0.008 & 3.301 & 0.001 & 3.685 & -0.033 & 2.231 & -0.010 & 16.343 \\ 
B5\_05 & -0.027 & 3.271 & -0.014 & 3.425 & -0.023 & 2.214 & -0.037 & 15.898 \\ 
B5\_06 & -0.047 & 3.291 & -0.016 & 3.548 & -0.038 & 2.159 & -0.052 & 19.485 \\ 
\textbf{B5\_mean} & \textbf{-0.050} & \textbf{3.363} & \textbf{-0.029} & \textbf{3.500} & \textbf{-0.054} & \textbf{2.219} & \textbf{-0.010} & \textbf{21.909} \\ 
\textbf{Overall} & \textbf{-0.045} & \textbf{3.368} & \textbf{-0.017} & \textbf{15.63} & \textbf{-0.033} & \textbf{2.578} & \textbf{-0.024} & \textbf{36.329} \\ 
\bottomrule
\end{tabular}
}
\end{table}



\begin{table}[ht]
\centering
\caption{\textbf{O4: Smoothness assessment based on the absolute angular acceleration and linear acceleration.} $\alpha_{abs} =| \frac{d^{2}\theta}{dt^{2}} |$: Angular acceleration ($deg/s^{2}$); $a_{abs} = | \frac{dv}{dt} |$: Linear acceleration ($m/s^{2}$). $R_{\alpha}, R_{a}$: ratio between the maximum value and average value. For simplicity, the suffix $abs$ is omitted in the Table.}
\label{tab:O4_detail}
\vspace{-2ex}
\scalebox{0.73}{
\begin{tabular}{lcccccc}
\toprule
& \( \bar{\alpha} \) & $\alpha_{max}$ & $R_{\alpha}$ & \( \bar{a} \) & $a_{max}$ & $R_{a}$ \\
\midrule
B1\_01  &  0.19  &  3.59  &  1874.52\%  &  0.000540  &  0.55  &  101731.88\% \\
B1\_02  &  0.33  &  5.67  &  1712.12\%  &  0.000004  &  1.18  &  27489802.25\% \\
B1\_03  &  0.36  &  4.42  &  1231.22\%  &  0.002251  &  1.02  &  45308.67\% \\
B1\_04  &  0.28  &  9.16  &  3326.23\%  &  0.004297  &  3.06  &  71290.39\% \\
B1\_05  &  0.20  &  2.22  &  1107.11\%  &  0.007219  &  4.91  &  67990.91\% \\
B1\_06  &  0.10  &  3.03  &  3124.59\%  &  0.000448  &  0.44  &  98933.73\% \\
\textbf{B1\_mean} & \textbf{0.24} & \textbf{4.68} & \textbf{2062.63\%} & \textbf{0.002460} & \textbf{1.86} & \textbf{4645842.97\%} \\
B2\_01  &  1.87  &  29.45  &  1573.91\%  &  0.025257  &  2.52  &  9965.94\% \\
B2\_02  &  1.07  &  11.92  &  1114.21\%  &  0.036006  &  1.11  &  3080.57\% \\
B2\_03  &  2.85  &  27.91  &  978.59\%  &  0.078414  &  3.69  &  4700.44\% \\
B2\_04  &  0.72  &  7.29  &  1011.68\%  &  0.018485  &  1.03  &  5571.57\% \\
B2\_05  &  0.99  &  26.08  &  2633.36\%  &  0.035711  &  0.65  &  1816.75\% \\
B2\_06  &  0.80  &  16.68  &  2084.46\%  &  0.026349  &  1.15  &  4348.28\% \\
\textbf{B2\_mean} & \textbf{1.38} & \textbf{19.89} & \textbf{1566.03\%} & \textbf{0.036704} & \textbf{1.69} & \textbf{4913.93\%} \\
B3\_01  &  0.54  &  9.04  &  1667.08\%  &  0.012594  &  3.05  &  24253.96\% \\
B3\_02  &  2.14  &  70.94  &  3322.51\%  &  0.179941  &  18.12  &  10067.54\% \\
B3\_03  &  3.00  &  81.16  &  2708.00\%  &  0.030535  &  15.72  &  51496.11\% \\
B3\_04  &  2.06  &  42.32  &  2056.36\%  &  0.184999  &  11.30  &  6107.04\% \\
B3\_05  &  0.93  &  10.33  &  1105.14\%  &  0.003369  &  2.00  &  59339.56\% \\
B3\_06  &  0.80  &  16.93  &  2109.13\%  &  0.002867  &  2.29  &  79793.00\% \\
\textbf{B3\_mean} & \textbf{1.58} & \textbf{38.45} & \textbf{2161.37\%} & \textbf{0.069051} & \textbf{8.75} & \textbf{38509.53\%} \\
B4\_01  &  1.29  &  12.30  &  951.80\%  &  0.057955  &  2.25  &  3887.62\% \\
B4\_02  &  1.32  &  11.74  &  890.71\%  &  0.070442  &  2.95  &  4181.80\% \\
B4\_03  &  1.03  &  11.77  &  1146.52\%  &  0.050847  &  3.81  &  7500.00\% \\
B4\_04  &  0.49  &  3.29  &  679.27\%  &  0.054317  &  1.48  &  2731.77\% \\
B4\_05  &  0.70  &  3.73  &  534.03\%  &  0.050300  &  3.27  &  6507.91\% \\
B4\_06  &  0.67  &  8.90  &  1325.34\%  &  0.027304  &  3.49  &  12764.99\% \\
\textbf{B4\_mean} & \textbf{0.92} & \textbf{8.62} & \textbf{921.28\%} & \textbf{0.051861} & \textbf{2.88} & \textbf{6262.35\%} \\
B5\_01  &  1.24  &  18.99  &  1530.36\%  &  0.069656  &  1.13  &  1622.05\% \\
B5\_02  &  1.29  &  12.95  &  1000.88\%  &  0.057046  &  2.96  &  5181.87\% \\
B5\_03  &  1.34  &  25.81  &  1924.76\%  &  0.067297  &  2.06  &  3055.69\% \\
B5\_04  &  0.70  &  3.74  &  533.25\%  &  0.054130  &  2.96  &  5465.59\% \\
B5\_05  &  0.64  &  4.64  &  721.43\%  &  0.041381  &  2.56  &  6193.42\% \\
B5\_06  &  0.66  &  5.13  &  772.38\%  &  0.042946  &  3.19  &  7418.08\% \\
\textbf{B5\_mean} & \textbf{0.98} & \textbf{11.88} & \textbf{1080.51\%} & \textbf{0.055409} & \textbf{2.48} & \textbf{4822.78\%} \\
\textbf{Overall} & \textbf{1.02} & \textbf{16.70} & \textbf{1558.36\%} & \textbf{0.043097} & \textbf{3.53} & \textbf{940070.31\%} \\
\bottomrule
\end{tabular}
}
\end{table}












\begin{figure*}[t] % horizontal figs
    \centering
    
    \subfigure[X position error]{
    \begin{minipage}[b]{0.19\textwidth}
    \includegraphics[scale=0.28]{fig/appendix/fixes/comparison_x.pdf}
    \centering
    \end{minipage}}
    \subfigure[Y position error]{
    \begin{minipage}[b]{0.19\textwidth}
    \includegraphics[scale=0.28]{fig/appendix/fixes/comparison_y.pdf}
    \centering
    \end{minipage}}
    \subfigure[Velocity error]{
    \begin{minipage}[b]{0.19\textwidth}
    \includegraphics[scale=0.28]{fig/appendix/fixes/comparison_v.pdf}
    \centering
    \end{minipage}}
    \subfigure[Acceleration error]{
    \begin{minipage}[b]{0.19\textwidth}
    \includegraphics[scale=0.28]{fig/appendix/fixes/comparison_a.pdf}
    \centering
    \end{minipage}}
    \subfigure[Heading angle error]{
    \begin{minipage}[b]{0.19\textwidth}
    \includegraphics[scale=0.28]{fig/appendix/fixes/comparison_theta.pdf}
    \centering
    \end{minipage}}


\vspace{-1.5ex}
\caption{\emph{Fixed controller}: Visualization of the Tracking Error (Error): X-axis is the timestamp and Y-axis is the state value, including position (subfigure (a) and (b)), velocity (c), acceleration (d) and heading angle (e).}
\vspace{-1ex}
\label{fig:fixed_O1_Assessment}
\end{figure*}





\begin{figure}[t]
\centering
\includegraphics[width = 1\linewidth]{fig/appendix/fixes/trajectory_plot_zoomed.pdf}
\centering
\vspace{-3ex}
\caption{\emph{Fixed controller:} Comparison between the planned trajectory and the actual trajectory.}
\label{fig:fixed_O1_traj_compare}
\vspace{-2.5ex}
\end{figure}





\subsection{Evaluating Fixed Controller}
\label{appendix:fixed_code}

We have tried to fix all control-related bugs in Tab.\ref{tab:identified_bugs}, and performed one round of oracle assessment (O1) based on this \emph{fixed controller}.
%
Particularly, the visualization of the results are shown in Fig.\ref{fig:fixed_O1_Assessment} and Fig.\ref{fig:fixed_O1_traj_compare}.
%
Comparing Fig.\ref{fig:fixed_O1_Assessment}.(c) with Fig.\ref{fig:O1_Assessment}.(c), it can be observed that the fixed controller has much better responsiveness on following the planned velocity.
%
Moreover, Comparing Fig.\ref{fig:fixed_O1_traj_compare} and Fig.\ref{fig:O1_traj_compare}, it is seen that the planned and actual trajectories are closer in Fig.\ref{fig:fixed_O1_traj_compare} than in Fig.\ref{fig:O1_traj_compare}, indicating a lower tracking error and better accuracy for our fixed controller.



%Comparing Fig.\ref{fig:fixed_O1_Assessment} and Fig.\ref{fig:O1_Assessment}




%Fig.\ref{fig:fixed_O1_Assessment} and Fig.\ref{fig:fixed_O1_traj_compare}.
